# Supplementary material for: Predicting the outcomes of treatment to eradicate the latent reservoir for HIV-1
Source: arXiv:1403.4196 ancillary file (2014-08-05)
Supplement: Supplementary file 1 [file SI.pdf]

# Supplementary Information

---

## Predicting the outcomes of treatment to eradicate the latent reservoir for HIV-1

Alison L. Hill[1,2,*], Daniel I. S. Rosenbloom[1,3,*], Feng Fu[4], Martin A. Nowak[1], and Robert F. Siliciano[5,†]

[1]Program for Evolutionary Dynamics, Department of Mathematics,Department of Organismic and Evolutionary Biology, Harvard University, Cambridge, MA 02138, USA
[2]Biophysics Program and Harvard-MIT Division of Health Sciences and Technology, Harvard University, Cambridge, MA 02138, USA
[3]Department of Biomedical Informatics, Columbia University Medical Center, New York, NY 10032, USA
[4]Institute of Integrative Biology, ETH Zurich, 8092 Zurich, Switzerland
[5]Department of Medicine, Johns Hopkins University School of Medicine and Howard Hughes Medical Institute, Baltimore, MD 21205, USA
[*]These authors contributed equally to the manuscript
[†]To whom correspondence should be addressed: rsiliciano@jhmi.edu

# Contents

**1 Stochastic model of viral dynamics** **2**
1.1 Notes on model choice . . . 2
1.2 Generating function analysis and clearance probability . . . 2
1.3 Simplified branching process . . . 3
1.4 Rebound time . . . 3
1.5 Expansion of the probability generating function . . . 5
1.6 Efficient computation of rebound probability . . . 6

**2 Estimating key parameters** **7**
2.1 Estimation of $\delta$ . . . 7
2.2 Estimation of $r$ . . . 7
2.3 Estimation of $A$ . . . 8
2.4 Estimation of $P_{Est}$ . . . 9
2.5 Estimation of the cell-to-virus ratio . . . 11

**3 Analysis of alternate stochastic models** **12**
3.1 Summary of alternate models . . . 12
3.2 Constant burst model . . . 13
3.3 Eclipse phase model . . . 13
3.4 Free virus model . . . 14
3.5 Homeostatic proliferation . . . 15
3.6 Bursting homeostatic proliferation . . . 16
3.7 Expansion upon reactivation . . . 17

# 1 Stochastic model of viral dynamics

## 1.1 Notes on model choice

Our model has similarities to other stochastic models of viral dynamics [1; 2] and to stochastic epidemiologic models that attempt to capture the variation in secondary infections between infected individuals [3; 4]. These models generally allow only a single event to happen to infected individuals (infection), and they explicitly specify the number of secondary infections by a Poisson (or other) distribution. We have extended this framework to be more consistent with well-validated differential equation-based models of viral dynamics by addition of a death term $d$. We believe that it is more realistic to include a separate death term for two main reasons: First, many events other than viral release lead to cell death, such as lysis by CD8$^+$ T cells. Second, deficiencies upstream of virion production – such as errors in reverse transcription or insufficient production of Tat to transactivate production of later proteins [5] – preclude production of any infectious virus. These mechanisms are not adequately captured in the term $p_\lambda(0)$, which represents only the Poisson probability that each virion independently fails to infect a cell. Inclusion of this death term allows for greater-than-Poisson variation in the total infection output of cells, which influences parameter $P_{Est}$ (see Section 2.4). Note that cells with nonviable provirus [6] are treated as dead in the model, as they cannot contribute to rebound.

## 1.2 Generating function analysis and clearance probability

Let $f_0(\xi_0, \xi_1; t)$ and $f_1(\xi_0, \xi_1; t)$ be probability generating functions for the process described in Methods starting from one latent and one active cell, respectively. Here, $\xi_0$ and $\xi_1$ are the dummy variables corresponding to the number of latent cells ($\mathcal{Y}(t)$) and active cells ($\mathcal{Z}(t)$), respectively, and $t$ is time since treatment interruption. The backwards Kolmogorov equations [7] are given by the system of coupled ordinary differential equations

$$\begin{aligned} \frac{\partial f_0}{\partial t} &= a(f_1 - f_0) + d_z(1 - f_0), \\ \frac{\partial f_1}{\partial t} &= b(\exp[\lambda(f_1 - 1)] - f_1) + d(1 - f_1), \end{aligned} \tag{S1}$$

with boundary conditions $f_0(\xi_0, \xi_1; 0) = \xi_0$ and $f_1(\xi_0, \xi_1; 0) = \xi_1$. The birth term $\exp(\lambda(f_1 - 1))$ follows from the Poisson offspring distribution with parameter $\lambda$.

After LRA therapy, the initial reservoir size $\mathcal{Z}(0)$ is Poisson-distributed with mean $qN_{LR}$. The initial number of actively infected cells was treated as Poisson-distributed around $aqN_{LR}/(b + d)$, representing activation-death equilibrium during effective treatment (birth events failing to produce new infected cells) with latently infected cells held constant at $qN_{LR}$. The probability generating function corresponding to this

initial condition is

$$f(\xi_0, \xi_1; t) = \exp\left[qN_{LR}\left(f_0\left(\xi_0, \xi_1; t\right) - 1\right) + \frac{aqN_{LR}}{b+d}\left(f_1\left(\xi_0, \xi_1; t\right) - 1\right)\right]. \tag{S2}$$

The fixed points of the differential equations (S1) give the extinction probabilities starting with one latent cell and one productive cell, respectively, denoted $P_{Clr|\mathcal{Z}=1}$ and $P_{Clr|\mathcal{Y}=1}$. The extinction probability starting from the actual initial conditions, denoted $P_{Clr}$, then equals $f(\xi_0, \xi_1; t)$ with the substitutions $f_0(\xi_0, \xi_1; t) = P_{Clr|\mathcal{Z}=1}$ and $f_1(\xi_0, \xi_1; t) = P_{Clr|\mathcal{Y}=1}$:

$$P_{Clr} = \exp\left[-aqN_{LR}\left(1 - P_{Clr|\mathcal{Y}=1}\right)\frac{b+d+a+d_z}{(b+d)(a+d_z)}\right] \approx \exp\left[-\frac{aqN_{LR}\left(1 - P_{Clr|\mathcal{Y}=1}\right)}{a+d_z}\right], \tag{S3}$$

where the approximation follows from the fact that rates controlling productive cells ($b$ and $d$) are much larger than rates controlling latent cells ($a$ and $d_z$). Parameters $b$, $d$, $a$, and $d_z$ can be replaced with the parameters estimated in Table 1, using the relationships $r = b\lambda - d$, $P_{Est} = 1 - P_{Clr|\mathcal{Y}=1}$, $\delta = a + d_z$, and $A = aN_{LR}$. Then $qA$ is the rate at which activated cells are produced, after therapy. The approximation of $P_{Clr}$ in (S3) becomes $\exp\left[-qAP_{Est}/\delta\right]$, consistent with [1].

### 1.3 Simplified branching process

Obtaining an explicit formula for rebound probability at a given time is not feasible in the above system. From here on we use a simplified branching process in which each birth event results in exactly two cells. Latent cell dynamics following interruption were the same as in the model described above. The differential equation for $f_1(\xi_0, \xi_1; t)$ is then

$$\frac{\partial f_1}{\partial t} = b\left(f_1\left(\xi_0, \xi_1; t\right)^2 - f_1\left(\xi_0, \xi_1; t\right)\right) + d\left(1 - f_1\left(\xi_0, \xi_1; t\right)\right), \tag{S4}$$

while the equation for $f_0(\xi_0, \xi_1; t)$ is unchanged. In this simplified process, $P_{Clr|\mathcal{Y}=1} = d/b$ and $r = b - d$. Computation of clearance probability proceeds as above, and the result in (S3) is unchanged.

### 1.4 Rebound time

The system with simplified replication dynamics (S4) can be solved explicitly:

$$
\begin{aligned}
f_0\left(\xi_0, \xi_1; t\right) &= 1 - a\frac{1-e^{-\delta t}}{\delta} + ae^{-\delta t}\int\limits_0^t e^{\delta\tau} f_1\left(\xi_0, \xi_1; \tau\right) \mathrm{d}\tau, \\
f_1\left(\xi_0, \xi_1; t\right) &= \frac{\left(1-P_{Est}\right)\left(e^{rt}\left(1-\xi_1\right)-1\right)+\xi_1}{-\left(1-P_{Est}\right)+e^{rt}\left(1-\xi_1\right)+\xi_1}.
\end{aligned}
\tag{S5}
$$

Let $f\left(\xi_0, \xi_1; t\right)$ be the generating function for the initial conditions described in 1.2, above. As rebound is defined only by the number of actively infected cells, it suffices to analyze the marginal generating function $f\left(1, \xi_1; t\right)$. From here on, the term $\xi_0$ is suppressed and $\xi_1$ is replaced with $\xi$:

$$
f\left(\xi; t\right) = \exp\left[qN_{LR}\left(f_0\left(\xi; t\right)-1\right) + \frac{aqN_{LR}P_{Est}}{r\left(2-P_{Est}\right)}\left(f_1\left(\xi; t\right)-1\right)\right]. \tag{S6}
$$

Assuming that active cell dynamics are much faster than latent cell dynamics (small $\delta/r$, to first-order), an explicit formula can be given for the expansion of the generating function $f\left(\xi; t\right)$ at $\xi = 0$. This expansion yields $P(\mathcal{Y}, t)$, the probability that there are exactly $\mathcal{Y}$ actively infected cells at time $t$ (see Section 1.5, below, for derivation):

$$
\begin{aligned}
P(\mathcal{Y}, t) \approx & \exp\left[-qAP_{Est}\left(\omega_1 + \frac{1-e^{\delta t}\left(1+\delta\int_0^t g(0;\tau)\mathrm{d}\tau\right)}{\delta P_{Est}}\right)\right] \\
& \times\frac{1}{\mathcal{Y}!}\left(\frac{e^{rt}-1}{e^{rt}-1+P_{Est}}\right)^{\mathcal{Y}} \\
& \times\left(\omega_2\right)_{\mathcal{Y}}\ M\left(-\mathcal{Y}, \omega_2, -\frac{qAP_{Est}^2}{2-P_{Est}}\omega_1\right),
\end{aligned}
\tag{S7}
$$

where $\omega_1 = \left(e^{rt}P_{Est}\right)/\left(r\left(e^{rt}-1\right)\left(e^{rt}-1+P_{Est}\right)\right)$, $\omega_2 = \left(qAP_{Est}e^{-\delta t}\right)/r$, $g(t) = e^{\delta t}\left(e^{rt}-1\right)\left(1-P_{Est}\right)/\left(e^{rt}-1+P_{Est}\right)$, $\left(\omega_2\right)_{\mathcal{Y}}$ uses the Pochhammer symbol (rising factorial), and $M$ is Kummer's confluent hypergeometric function. Note that unlike with standard techniques for inverting generating functions [8; 9], the integrand on the first line of (S7) is not a highly oscillatory function, and so numerical computation is efficient.

Let $P(\geq N_{Reb}, t)$ be the probability of rebound, defined as there being at least $N_{Reb}$ actively infected cells at time $t$. Direct computation of this quantity as $1-\sum_{\mathcal{Y}=0}^{N_{Reb}-1} P(\mathcal{Y}, t)$ is relatively slow. In Section 1.6, below, we show that for realistically large $N_{Reb}$, this probability can be efficiently computed as

$$
P(\geq N_{Reb}, t) \approx \left(1-P_{Clr}\right)\frac{\int_0^t P(N_{Reb}, \tau)\,\mathrm{d}\tau}{\int_0^\infty P(N_{Reb}, \tau)\,\mathrm{d}\tau}. \tag{S8}
$$

A script is provided at `http://www.danielrosenbloom.com/reboundtimes` using this formula for rapid computation of survival curves.

### 1.5 Expansion of the probability generating function

The generating function (S6) can be written

$$f\left(\xi;t\right)=\exp\left[k_1+b_1 g_1\left(\xi;t\right)+b_2\int\limits_0^t g_2\left(\xi;\tau\right)\,\mathrm{d}\tau\right], \tag{S9}$$

where

$$\begin{aligned} k_1 &= -\left(\frac{qA}{\delta}\right)\left(1-e^{-\delta t}\right), \\ b_1 &= -\frac{qAP_{Est}^2 e^{rt}}{r\left(2-P_{Est}\right)}, \\ b_2 &= qAe^{-\delta t}, \\ g_1(\xi;t) &= \frac{1-\xi}{\left(e^{rt}-1\right)\left(1-\xi\right)+P_{Est}}, \\ g_2(\xi;t) &= e^{\delta t}\frac{\left(e^{rt}-1\right)\left(1-\xi\right)\left(1-P_{Est}\right)+P_{Est}\xi}{\left(e^{rt}-1\right)\left(1-\xi\right)+P_{Est}}. \end{aligned} \tag{S10}$$

The derivatives of $g_1(\xi;t)$ and $g_2(\xi;t)$ at $\xi=0$ can be written explicitly:

$$\begin{aligned} g_1(0;t) &= \frac{1}{e^{rt}-1+P_{Est}}, \\ g_2(0;t) &= e^{\delta t}\frac{\left(e^{rt}-1\right)\left(1-P_{Est}\right)}{e^{rt}-1+P_{Est}}, \\ \left.\frac{\partial^j g_1(\xi;t)}{\partial\xi^j}\right|_{\xi=0} &= -j!\,\frac{\left(e^{rt}-1\right)^{j-1}P_{Est}}{\left(e^{rt}-1+P_{Est}\right)^{j+1}}, \\ \left.\frac{\partial^j g_2(\xi;t)}{\partial\xi^j}\right|_{\xi=0} &= j!\,e^{(r+\delta)t}\left(\frac{e^{rt}-1}{e^{rt}-1+P_{Est}}\right)^{j-1}\left(\frac{P_{Est}}{e^{rt}-1+P_{Est}}\right)^2, \end{aligned} \tag{S11}$$

for all $j>0$.

Note that $g_2(\xi;t)$ and its derivatives contribute to the generating function (S9) only via integration over $\tau$ from 0 to $t$. In the limit of large $\tau$, the derivative $\left.\frac{\partial^j g_2(\xi,\tau)}{\partial\xi^j}\right|_{\xi=0}$ approaches $j!\,e^{(-r+\delta)\tau}P_{Est}^2$ for any $j>0$. Assuming that active cell dynamics are faster than latent cell dynamics, $\delta$ is much smaller than $r$, and so this derivative vanishes as $r\tau$ grows. It therefore contributes meaningfully to the integral only at small $r\tau$, a regime in which $e^{\delta t}\approx 1$. For the purposes of calculating the generating function expansion, we therefore may safely ignore $\delta$ in the derivatives of $g_2(\xi;t)$, arriving at the approximation

$$\left.\frac{\partial^j g_2(\xi,t)}{\partial \xi^j}\right|_{\xi=0} \approx j!\, e^{rt} \left(\frac{e^{rt}-1}{e^{rt}-1+P_{Est}}\right)^{j-1} \left(\frac{P_{Est}}{e^{rt}-1+P_{Est}}\right)^2 \qquad (\delta \ll r \text{ and } j>0). \tag{S12}$$

Let $P(\mathcal{Y},t)$ denote the probability that $\mathcal{Y}$ active cells are present at time $t$. This probability equals the coefficient of $\xi^{\mathcal{Y}}$ in the expansion of $f(\xi;t)$ around $\xi=0$, which is $\frac{1}{\mathcal{Y}!}\left.\frac{\partial^{\mathcal{Y}} f(\xi;t)}{\partial \xi^{\mathcal{Y}}}\right|_{\xi=0}$. Using approximation (S12), the expansion is

$$\begin{aligned} P(\mathcal{Y},t) \approx & \frac{1}{\mathcal{Y}!\ (e^{rt}-1+P_{Est})^{2\mathcal{Y}}} e^{k_1+b_1/\left(e^{rt}-1+P_{Est}\right)+b_2\int_0^t g_2(0;\tau)\mathrm{d}\tau} \\ \times & \sum_{i=0}^{\mathcal{Y}} \binom{\mathcal{Y}}{i} (-b_1 P_{Est})^i \left(\left(e^{rt}-1\right)\left(e^{rt}-1+P_{Est}\right)\right)^{\mathcal{Y}-i} \\ & \left(\frac{b_2 P_{Est}}{r}+i\right)_{\mathcal{Y}-i}. \end{aligned} \tag{S13}$$

Expression (S7) in the previous section is a more convenient formulation of this probability in terms of a hypergeometric polynomial.

## 1.6 Efficient computation of rebound probability

Rebound probability $P(\geq N_{Reb},t)$ is the probability that there are at least $N_{Reb}$ active cells at time $t$. Define $P(\geq N_{Reb},\infty)$ as the probability that rebound *ever* occurs. Since realistic values of $N_{Reb}$ are large (many thousands of infected cells), $P(\geq N_{Reb},\infty)$ is approximately one minus the extinction probability, given in (S3).

Also since $N_{Reb}$ is large, we can assume that, once this rebound level is achieved, the number of active cells is almost always increasing; that is, decreases are rare and short-lived. The probability $P(\geq N_{Reb},t)$ is therefore nearly equal to the probability that there were *ever* exactly $N_{Reb}$ cells sometime prior to $t$. Define $E(N_{Reb},t) = \int_0^t P(N_{Reb},\tau)\mathrm{d}\tau$, the expected duration for which exactly $N_{Reb}$ cells existed, prior to $t$. This expectation can be decomposed $E(N_{Reb},t) \approx P(> N_{Reb},t)D(N_{Reb})$, where $D(N_{Reb})$ is the expected duration that the number of active cells stays at $N_{Reb}$ conditional upon it reaching $N_{Reb}$. Again by large $N_{Reb}$, this duration is insensitive to latent cell dynamics and so is independent of time. Similarly, let $E(N_{Reb},\infty) = \int_0^\infty P(N_{Reb},\tau)\mathrm{d}\tau$, which is approximately $P(> N_{Reb},\infty)D(N_{Reb})$. The desired probability is therefore $P(\geq N_{Reb},t) \approx P(> N_{Reb},\infty)E(N_{Reb},t)/E(N_{Reb},\infty) \approx (1-P_{Clr})\,E(N_{Reb},t)/E(N_{Reb},\infty)$, as given in equation (S8).

## 2 Estimating key parameters

### 2.1 Estimation of $\delta$

The net decay rate of the latent reservoir ($\delta$) was estimated from a previous study of longitudinal reservoir size in patients on long-term ART. Table 1 of Siliciano *et al.*[10] reports the mean and 95% confidence interval of LR decay from a cohort of 59 patients, derived using a mixed-effects model. This method models each patient's decay rate $\delta_i$ as being sampled from a population-level normal distribution with mean $5.2 \times 10^{-4}$ d$^{-1}$ and standard deviation of $1.6 \times 10^{-4}$ d$^{-1}$. We use this distribution to sample simulated patients. Note that with this method, approximately 1 in 1500 draws will give a negative value of $\delta$, corresponding to an LR that fails to decay (e.g., by homeostatic proliferation outweighting activation plus death). We allowed negative $\delta$ only for simulation of the model with homeostatic proliferation; for all others, we truncated the distribution at zero.

The mean decay rate from the Siliciano study corresponds to a reservoir half-life of 44 months, which is consistent with a more recent study that found a value of 43 months [11].

### 2.2 Estimation of $r$

The net exponential growth rate of the infection ($r$) and the number of latent cells reactivating per day ($A$) before reservoir-reducing therapy can be estimated from ART-interruption studies. Luo *et al.* [12] report the joint posterior distributions of viral dynamic parameters for 10 patients who underwent 3-5 structured treatment interruptions in a previous study[13]. From these, we computed inter-patient distributions for both $r$ and $A$.

The authors used a system of three differential equations to describe viral rebound during treatment interruption: $\dot{x}(t) = \lambda_x - d_x x(t) - \beta x(t)v(t)$, $\dot{y}(t) = \beta x(t)v(t) - d_y y(t) + \lambda_y$, and $\dot{v}(t) = \gamma y(t) - d_v v(t)$; where state variables $x$, $y$, and $v$ represented plasma concentrations of uninfected CD4$^+$ T cells, productively infected CD4$^+$ T cells, and free virus, respectively. Parameters $\lambda_x$ and $d_x$ denote production and death rates of target cells, respectively; $\beta$ is infectivity; $d_y$ is the total death rate of infected cells; $\gamma$ is the viral production rate by infected cells; $d_v$ is the viral clearance rate; and $\lambda_y$ represents the rate at which latently infected cells activate to become productively infected cells.

The desired parameter $r$ is the net growth rate of the infection at low viral loads, and in terms of the paper's model, corresponds to: $r = (\beta\lambda\gamma)/(d_x d_v) - d_y$. To estimate the population-level posterior distribution for $r$, we used the paper's reported posterior distributions of the basic parameters for each patient. They reported these distributions as a list of 200,000 samples for each patient, from which we ignored the first 50,000 to allow convergence and used the remaining 150,000 as the individual-level posterior estimate for that patient. We then treated each posterior estimate of $\log(r)$ as a random normal variable sampled

from $\mathcal{N}(\mu_i, \sigma_i)$, where each patient's $\mu_i$ is sampled from $\mathcal{N}(\mu, \sigma)$. Population parameters were estimated by maximum likelihood using the `mvmeta` library in R to be $\mu = -0.398$ and $\sigma = 0.194$. The geometric mean of the corresponding lognormal distribution therefore corresponds to $r = 0.4$ d$^{-1}$.

We confirmed these values with data from a separate treatment interruption trial[14], using a least-squares fit to exponential growth of viral load shortly after rebound. This analysis again produced a geometric mean value of $r = 0.4$ d$^{-1}$.

Another commonly used measure of viral fitness is the basic reproductive ratio $R_0$, which describes the average number of new cells infected by virus from a single actively infected cell. The growth rate and the basic reproductive ratio relate to each other as $R_0 = r/d_y + 1$, where $d_y = b + d$. Using the well-established average lifespan of infected CD4$^+$ T cells of 1 day (measured from viral load decay during ART [15]) a growth rate of $r = 0.4$ corresponds to $R_0 = 1.4$. This basic reproductive ratio observed during ART interruption is consistently lower than that observed during acute infection (for which $R_0 \approx 8-10$)[16; 17], likely due to improved immune response.

In using the above analysis to estimate $r$, we have assumed that the growth rate of a reactivating viral lineage does not change between the time of ART/LRA interruption and the detection of viral rebound. Three mechanisms might cause this parameter to vary. First, as the waiting time to latent cell reactivation increases, the fitness of the reactivated virus may increase, since CTL responses could have waned in the absence of antigen. To account for waning immunity, one could allow parameters $r$ and $P_{Est}$ to drift upwards slowly over time, potentially hastening rebound in the activation-limited regime. Although the worst-case value for $r$ is likely to be the growth rate observed during acute infection, it is unclear how to estimate the particular time-dependence from existing treatment interruption studies, as successful LRA may reduce antigenic stimulus to a level below that of ART alone. Second, once rebound starts, viral growth rate could decrease over time as the immune response is activated, leading to sub-exponential growth. Studies of repeated treatment interruptions that have characterized changes in growth rate and CTL responses suggest that this effect is minor [18]. Finally, cooperative growth effects, perhaps due to antigen-driven immune activation, could drive up $r$ as the infection size grows, but measuring such an effect *in vivo* is currently impossible. In the absence of clear evidence for the three effects, we have assumed the simplest scenario of constant parameter values.

## 2.3 Estimation of $A$

We use the Luo *et al.* [12] data and a similar procedure to estimate $A$, the number of cells exiting the LR per day during fully suppressive ART, which is proportional to the initial residual viral load from which rebound begins. As this data included densely sampled viral load, but few measurements of CD4$^+$ T cells, the fitted parameters are most reliable in determining virological quantities, not cell counts. For example, the quantity $(\gamma\lambda_y)/(d_v d_y)$, which equals the residual viral load observed during fully suppressive therapy,

should be particularly reliable. Additionally, $d_y$ itself can be reliably determined the decay of viral load upon resumption of therapy [15]. Since it is the product of two reliable parameters, the rate of virus production during ART ($\lambda_v = (\gamma \lambda_y)/d_v$) will also be a reliable quantity to estimate. In contrast, the cellular rate $\lambda_y$ by itself may not be reliably estimated from this data. In fact, since Luo *et al.*[12] identified the sum $x(t) + y(t)$ with *total* CD4 count, though the majority of CD4$^+$ T cells are not actually infectable, they should systematically report an *overestimate* of parameter $\lambda_y$. We therefore felt that $A$ could be estimated more robustly by exploiting its proportionality to reliably estimated viral rates.

We estimate $A$ in two steps: (1) use the posterior distributions reported by Luo *et al.*[12] to estimate the interpatient distribution for $\lambda_v$, which has units of copies of viral RNA per ml plasma, per day; (2) use separate observations regarding the ratio of cells to virus to scale $\lambda_v$ to $A$, which has units of (total body) infected CD4$^+$ T cells per day. Analogously to the above estimation of $r$, we estimated a lognormal interpatient distribution for $\lambda_v$, obtaining log mean and standard deviation $-1.469$ and $0.991$, respectively. To scale to $A$, we used the cell-to-virus ratio described below, which implies that $A$ is $(750 \text{ to } 3750) \times \lambda_v$. To obtain a normal distribution for $\log(A)$, we treated the extremes of 750 and 3750 as estimates of the 95% CI for the ratio $A/\lambda_v$, adding $\frac{1}{2}(\log(750) + \log(3750)) = 3.225$ to the mean and $0.178$ to the standard deviation. The resulting distribution for $A$ has log mean and standard deviation 1.755 and 1.007, respectively.

### 2.4 Estimation of $P_{Est}$

Measuring establishment probabilities in early stages of infections is a difficult task that requires frequent tracking of rare infection and extinction events in small populations (e.g., Hofacre *et al.*[19]). In contrast, even the most sensitive methods currently used to measure growth of HIV over time *in vitro* do not yet provide single-cell resolution [20; 21]. In the absence of the relevant experimental results, we rely on population genetic models to estimate $P_{Est}$.

In the basic stochastic model described above, the establishment probability is mainly controlled by the parameter $\lambda$. For a fixed growth rate $r$, higher $\lambda$ values correspond to lower values of $P_{Est}$. To generalize this concept to measures more common in population genetics, we reframe $P_{Est}$ in terms of the quantity $\rho$ – the ratio of the variance to the mean offspring number for a single cell. In our basic model, $\rho = 1 + d\lambda/(b+d)$, as the mean offspring number (basic reproductive ratio) is $R_0 = b\lambda/(b+d)$ and the variance is $\left(b\left(\lambda + (\lambda - R_0)^2\right) + dR_0^2\right)/(b+d)$. Thus the establishment probability depends only on $\rho$ and $R_0$ and is the solution to

$$P_{Est}\,(R_0 + \rho - 1) = R_0\left(1 - e^{-P_{Est}(R_0+\rho-1)}\right). \tag{S14}$$

Using this equation we can use estimates of $\rho$ from various data sources to derive a range of reasonable values for $P_{Est}$.

The maximum establishment probability compatible with a fixed viral fitness $R_0$ occurs when $d = 0$, which sets $\rho = 1$ and results in $P_{Est}$ being determined by the equation $P_{Est} = 1 - e^{-P_{Est}R_0}$. This equation corresponds to the establishment probability relationship derived by Pennings [22] and by Pearson *et al.*[2] for their "burst model." Thus the $\rho = 1$ limit sets a natural upper bound for $P_{Est}$.

To estimate a lower bound for $P_{Est}$, note that the ratio $\rho$ measures the deviation of viral replication from a simple Poisson process. Population genetic studies have consistently measured the effective population size ($N_e$) of an individual host's infection as far smaller than the total number of cells infected with HIV ($N$) [23], an indication of greater-than-Poisson variance in the replication process. The ratio $N/N_e$ reports an order-of-magnitude estimate for $\rho$. Since equilibrium models of neutral diversity may not be applicable to a population such as HIV that undergoes frequent selective sweeps [23; 24], we consider two studies based on models of selective sweeps, both of which converge upon an estimate of $N_e \approx 10^5$ for patients on either no treatment or ineffective treatment [24; 25]. As others have pointed out [26], this value likely represents a lower bound on $N_e$, as opposed to a point estimate. Using $N \approx 10^8$ as a typical number of infected cells off therapy, which likely overestimates the total population size during any type of treatment, these studies imply $\rho \lesssim 10^3$.

Some care is required to interpret this value in the context of our model: since these studies examined diverse, evolving viral populations, strains with low relative fitness tend to contribute negligibly to $N_e$ [24]. In the small-infection regime of our model, however, relative fitness differences between strains are unimportant, and any virus that is viable (in the sense of absolute fitness, $r > 0$ or $R_0 > 1$) is capable of establishing a rebounding infection. This is yet another reason why the estimate $\rho \approx 10^3$ is a conservative upper bound for the true value of $\rho$, providing a lower bound for $P_{Est}$.

The most relevant estimate for the establishment probability to our knowledge comes from an analysis of the rate of emergence of drug-resistant variants from the latent reservoir during fully suppressive ART. This study calculated an "effective exit rate" from the latent reservoir of 5 productively infected cells per day [22]. When compared to our estimate of $A$ centered at 57 cells per day (Table 1), this implies $\rho \approx 57/5 = 11.4$. We therefore use $\rho \approx 10$ as the best parameter estimate and the center of sampled range.

To obtain an alternate estimate of $\rho$ based on *in vitro* evidence, we consider variance in viral gene expression. In an HIV-1-based fluorescent reporter gene system in a T cell culture line, Singh et al. [27] measured the distribution of gene expression levels across individual HIV-infected cells, in 30 different clones. Assuming that expression level is proportional to subsequent infection events, and that the viral transcriptional circuit is regulated similarly *in vitro* as *in vivo*, the ratio of the variance to the mean of gene expression provides an estimate for $\rho$. Singh et al. report that expression followed a modified Poisson law with excess variance, even when controlling for variation due to both integration site effects and positive-feedback effects driven by the viral protein Tat [5]. Their results were well described by a"burst" model of viral protein production, in which $\rho$ is equivalent to their "burst size," plus one. In their conservative estimates, variance in gene expression outstripped Poisson variation by up to 11-fold, with a majority of

clones showing a 3-fold increase. It is highly likely that additional sources of variation in infection not captured in this assay, such as Tat-based feedback, variation in translation and virion assembly, in viral fitness effects, or in the tissue microenvironment, would increase $\rho$ *in vivo*. This analysis therefore offers $\rho$ = 3 as a low estimate but is highly suggestive of larger $\rho$.

To capture the current state of knowledge and represent our uncertainty, we use a lognormal distribution for $\rho$ centered at 10 with 95% of the distribution falling between 1 and 100. After sampling $r$ and $\rho$, we compute $R_0$ (described above in the Section 2.2) and then $P_{Est}$ (using Eq. (S14)).

## 2.5 Estimation of the cell-to-virus ratio

Because the model tracks only infected cells, but must relate total body cell counts to clinically observed plasma viral RNA concentrations, we require an estimate of the conversion factor between these two quantities. For this calculation we applied a version of the analysis developed in De Boer *et al.* [28]. Let $\mathcal{Y}$ be the total body number of productively infected cells residing in lymphoid tissue, let $\mathcal{V}$ be the total body number of free virus particles, and let $\kappa$ be the per-cell production rate of virions. We can balance viral production and decay at equilibrium for a typical 70-kg indivivdual:

$$\begin{aligned}
\kappa\mathcal{Y} &= d_v\mathcal{V} \\
\mathcal{Y} &= \left(\frac{d_v}{\kappa}\right)\left(\frac{\text{100 virions in LT}}{\text{1 virion in ECF}}\right)\left(\frac{\text{1 virion in ECF}}{\text{2 RNA copies in ECF}}\right)(\text{15,000 ml ECF})\,v \\
&= \left(\frac{d_v}{\kappa}\right)\left(7.5\times10^5\,\frac{\text{virions in LT}}{\text{RNA copies per ml ECF}}\right)v,
\end{aligned} \tag{S15}$$

where $v$ is the per-ml concentration of viral RNA in circulation. Here we use the estimate that virus particles in the lymphoid tissue outnumber those in circulation 100-fold, mirroring the ratio of lymphocytes in lymph nodes versus in circulation [29; 30]. Note that since the lifespan of an infected cell is much longer than that of a free virion, the ratio of production to decay rates, $\kappa/d_v$, equals the number of free virions associated with a productive cell during most of that cell's existence; values of 200–1000 are consistent with recent experiments [28; 31; 32]. The resulting estimate for $\mathcal{Y}$ is therefore $(750 \text{ to } 3750) \times v$. We use the geometric mean of these values – 1680 – as a point estimate. With this value the viral rebound threshold of 200 c ml$^{-1}$corresponds to $\mathcal{Y} \approx 3 \times 10^5$. Note that model results are insensitive to this value, as rebound probability depends on the logarithm of the rebound threshold.

# 3 Analysis of alternate stochastic models

## 3.1 Summary of alternate models

The basic five-parameter, two-variable model described above was used to derive the result that the outcomes of reservoir-reducing therapy depend only on four "key parameters," which are not necessarily model-specific. To test the robustness of this claim to structural variation in model choice, we constructed a series of alternate stochastic models, some of which include more complex infection processes. For each model, we derived expressions relating the model-specific parameters to the four key parameters. We then simulated the model and compared it to simulations of the basic model with identical values of the key parameters. There is generally an infinite set of model-specific parameters satisfying the same key parameter values; where needed, we evaluated a few examples at the extremes of what could be considered biologically realistic. A full description of the models, parameters, and results is given in the following section. In summary, the alternate models were:

1. Constant burst model: Infected cells either die without infecting, or produce a fixed (integer) number of new infected cells.

2. Eclipse phase model: Upon reactivation from latency or new infection, cells enter an "eclipse phase" in which they cannot infect others (no virus is produced). Cells in the eclipse phase may either die or proceed to the productively infected phase, where they behave as infected cells do in the constant burst model. We consider a eclipse phase of average length 2 days with 1/6 chance of death.

3. Free virus model: We explicitly track the amount of free virus. Infected cells either die without infecting, or produce a fixed (integer) number of virions. Each virion may either be cleared or may infect a new cell. We consider viral burst sizes ranging from 10 to 1000 virions.

4. Homeostatic proliferation: Latently infected cells can either reactivate, die, or divide *without reactivating* giving rise to another latently infected cell. To test a reasonable biological limit of fast turnover, cells have an average lifespan of 6 months, but the net LR half-life is maintained at 44 months by proliferation.

5. Bursting homeostatic proliferation: Latently infected cells can either reactivate, die, or divide multiple times *without reactivating* giving rise to a burst of other latently infected cells. To test a biological limit of fast turnover, cells have an average lifespan of 6 months, but the net LR half-life is maintained at 44 months by proliferation with 4 divisions leading to 16 cells.

6. Expansion upon reactivation: When latently infected cells reactivate, they first proliferate multiple times *without infecting others*. Thus each reactivated latent cell results in multiple productively infected cells. We consider a maximum of 4 divisions leading to 16 newly reactivated cells.

### 3.2 Constant burst model

**Summary:** Infected cells either die without infecting, or produce a fixed (integer) number of new infected cells.

**Process:**

$$\begin{aligned} Z &\to Y \text{... rate constant: } a \\ Z &\to \emptyset \text{... rate constant: } d_z \\ Y &\to \lambda Y \text{... rate constant: } b \\ Y &\to \emptyset \text{... rate constant: } d \end{aligned} \tag{S16}$$

$Y$ and $Z$ are individual actively or latently infected cells. An actively infected cell can either die (at rate $d$) or produce a collection of virions (at rate $b$) that results in the infection of $\lambda$ other cells, where $\lambda$ is an integer. After an infection event, the original cell dies. Free virus is not explicitly tracked, but assumed to be at a level proportional to the number of actively infected cells. Latently infected cells can either die (at rate $d_z$) or reactivate and become productively infected (at rate $a$). All rates have units of d$^{-1}$, and $\lambda$ is unitless.

**Parameters:**

- $r = b\lambda - (b + d)$
- $A = aN_{LR}$
- $\delta = d_z + a$
- $P_{Est}$ is the solution to $R_0(1 - (1 - P_{Est})^{\lambda}) - \lambda P_{Est} = 0$
- $R_0 = \frac{b\lambda}{d_y}$, $d_y = (b + d)$

### 3.3 Eclipse phase model

**Summary:** Upon reactivation from latency or new infection, cells enter an "eclipse phase" in which they cannot infected others (no virus is produced). Cells in the eclipse phase have may either die or proceed to the productively infected phase, where they behave according to infected cells in the constant burst model. We consider a eclipse phase of 2-day average length with 1/6 chance of death.

**Process:**

$$
\begin{aligned}
Z &\rightarrow W\text{... rate constant: } a \\
Z &\rightarrow \emptyset\text{... rate constant: } d_z \\
W &\rightarrow Y\text{... rate constant: } e \\
W &\rightarrow \emptyset\text{... rate constant: } f \\
Y &\rightarrow \lambda W\text{... rate constant: } b \\
Y &\rightarrow \emptyset\text{... rate constant: } d
\end{aligned}
\tag{S17}
$$

$Y$ and $Z$ are individual productively or latently infected cells. $W$ is an early "eclipse" phase cell. A productively infected cell can either die (at rate $d$) or produce a collection of virions (at rate $b$) that results in the infection of $\lambda$ eclipse phase cells, where $\lambda$ is an integer. After an infection event, the original cell dies. Free virus is not explicitly tracked, but assumed to be at a level proportional to the number of productively infected cells. Eclipse phase cells can either die (at rate $f$) or proceed to the productively infected phase (at rate $e$). Latently infected cells can either die (at rate $d_z$) or reactivate and become eclipse phase cells (at rate $a$). All rates have units of d$^{-1}$, and $\lambda$ is unitless.

**Parameters**

- $r = (1/2)(-(d_w + d_y) + \sqrt{(d_w + d_y)^2 + 4d_w d_y(R_0 - 1)})$
- $A = aN_{LR}$
- $\delta = d_z + a$
- $P_{Est}$ is the solution to $R_0(1-(1-P_{Est})^\lambda) - \lambda P_{Est} = 0$ (this is the establishment probability starting from a single cell in the eclipse phase. For a single productively infected cell, $P^y_{Est} = \frac{d_w}{e} P_{Est}$.
- $R_0 = \frac{be\lambda}{d_w d_y}$, $d_w = e + f$, $d_y = b + d$

## 3.4 Free virus model

**Summary:** We explicitly track the amount of free virus. Infected cells either die without infectiong, or produce a fixed (integer) number of virions. Each virion may either be cleared or infected a new cell.

**Process:**

$$
\begin{aligned}
&Z \to Y\text{... rate constant: } a\\
&Z \to \emptyset\text{... rate constant: } d_z\\
&Y \to NV\text{... rate constant: } k\\
&Y \to \emptyset\text{... rate constant: } d\\
&V \to Y\text{... rate constant: } b\\
&V \to \emptyset\text{... rate constant: } c
\end{aligned}
\tag{S18}
$$

$Y$ and $Z$ are individual actively or latently infected cells. $V$ is a free virion. An actively infected cell can either die (at rate $d$) or produce a collection of virions (at rate $k$) that results in the production of $N$ virions, were $N$ is an integer. After an infection event, the original cell dies. Each free virion can either be cleared (at rate $c$) or infect another cell (at rate $b$). Latently infected cells can either die (at rate $d_z$) or reactivate and become productively infected (at rate $a$). All rates have units of day$^{-1}$, and $N$ is unitless.

**Parameters:**

- $r = (1/2)(-(d_v + d_y) + \sqrt{(d_v + d_y)^2 + 4d_v d_y(R_0 - 1)})$
- $A = aN_{LR}$
- $\delta = d_z + a$
- $P_{Est} = \frac{d_v}{b} P^v_{Est}$, where $P^v_{Est}$ is the solution to $R_0(1 - (1 - P^v_{Est})^N) - NP^v_{Est} = 0$ ($P_{Est}$ is the establishment probability starting from a single cell, and $P^v_{Est}$ is the establishment probability starting from a single virion.
- $R_0 = \frac{kbN}{d_v d_y}$, $d_v = b + c$, $d_y = k + d$

## 3.5 Homeostatic proliferation

**Summary:** Latently infected cells can either reactivate, die, or divide *without reactivating* giving rise to another latently infected cells.

**Process:**

$$
\begin{aligned}
&Z \to Y\text{... rate constant: } a\\
&Z \to \emptyset\text{... rate constant: } d_z\\
&Z \to 2Z\text{... rate constant: } p\\
&Y \to cY\text{... rate constant: } b \times p_\lambda(c)\\
&Y \to \emptyset\text{... rate constant: } d
\end{aligned} \tag{S19}
$$

$Y$ and $Z$ are individual actively or latently infected cells. An actively infected cell can either die (at rate $d$) or produce a collection of virions (at rate $b$) that results in the infection of $c$ other cells, where $c$ is a Poisson-distributed random variable with parameter $\lambda$, $p_\lambda(c) = \frac{\exp(-\lambda)\lambda^c}{c!}$. After an infection event, the original cell dies. Free virus is not explicitly tracked, but assumed to be at a level proportional to the number of actively infected cells. Latently infected cells can either die (at rate $d_z$), reactivate and become productively infected (at rate $a$), or divide *without reactivating* giving rise to another latently infected cell. All rates have units of day$^{-1}$, and $\lambda$ is unitless.

**Parameters:**

- $r = b\lambda - (b + d)$
- $A = aN_{LR}$
- $\delta = d_z + a - p$
- $P_{Est}$ is the solution to $R_0(1 - e^{-\lambda P_{Est}}) - \lambda P_{Est} = 0$
- $R_0 = \frac{b\lambda}{d_y}$, $d_y = (b + d)$

### 3.6 Bursting homeostatic proliferation

**Summary** Latently infected cells can either reactivate, die, or divide multiple times *without reactivating* giving rise to a burst of other latently infected cells.

**Process:**

$$
\begin{aligned}
&Z \to Y \text{... rate constant: } a \\
&Z \to \emptyset \text{... rate constant: } d_z \\
&Z \to 2^h Z \text{... rate constant: } p \\
&Y \to cY \text{... rate constant: } b \times p_\lambda(c) \\
&Y \to \emptyset \text{... rate constant: } d
\end{aligned}
\tag{S20}
$$

$Y$ and $Z$ are individual actively or latently infected cells. An actively infected cell can either die (at rate $d$) or produce a collection of virions (at rate $b$) that results in the infection of $c$ other cells, where $c$ is a Poisson-distributed random variable with parameter $\lambda$, $p_\lambda(c) = \frac{\exp(-\lambda)\lambda^c}{c!}$. After an infection event, the original cell dies. Free virus is not explicitly tracked, but assumed to be at a level proportional to the number of actively infected cells. Latently infected cells can either die (at rate $d_z$), reactivate and become productively infected (at rate $a$), or divide $h$ times *without reactivating* giving rise to $2^h$ latently infected cells (where $h$ is an integer). All rates have units of day$^{-1}$, and $\lambda$ and $h$ are unitless.

**Parameters:**

- $r = b\lambda - (b + d)$
- $A = aN_{LR}$
- $\delta = d_z + a - p(2^h - 1)$
- $P_{Est}$ is the solution to $R_0(1 - e^{-\lambda P_{Est}}) - \lambda P_{Est} = 0$
- $R_0 = \frac{b\lambda}{d_y}$, $d_y = (b + d)$

### 3.7 Expansion upon reactivation

**Summary:** When latently infected cells reactivate, they first proliferate multiple times *without infecting others*.

**Process:**

$$
\begin{aligned}
&Z \to 2^m Y \text{... rate constant: } a \\
&Z \to \emptyset \text{... rate constant: } d_z \\
&Y \to cY \text{... rate constant: } b \times p_\lambda(c) \\
&Y \to \emptyset \text{... rate constant: } d
\end{aligned}
\tag{S21}
$$

$Y$ and $Z$ are individual actively or latently infected cells. An actively infected cell can either die (at rate $d$) or produce a collection of virions (at rate $b$) that results in the infection of $c$ other cells, where $c$ is a Poisson-distributed random variable with parameter $\lambda$, $p_\lambda(c) = \frac{\exp(-\lambda)\lambda^c}{c!}$. After an infection event, the original cell dies. Free virus is not explicitly tracked, but assumed to be at a level proportional to the number of actively infected cells. Latently infected cells can either die (at rate $d_z$), or reactivate (at rate $a$) and proliferate $m$ times to produce $2^m$ actively infected cells (where $m$ is an integer). All rates have units of day$^{-1}$, and $\lambda$ and $m$ are unitless.

**Parameters:**

- $r = b\lambda - (b + d)$
- $A = a2^m N_{LR}$
- $\delta = d_z + a$
- $P_{Est}$ is the solution to $R_0(1 - e^{-\lambda P_{Est}}) - \lambda P_{Est} = 0$
- $R_0 = \frac{b\lambda}{d_y}$, $d_y = (b + d)$

# References


[1] Haeno, H. & Iwasa, Y. Probability of resistance evolution for exponentially growing virus in the host. *Journal of Theoretical Biology* **246**(2), 323–331, May (2007).

[2] Pearson, J. E., Krapivsky, P., & Perelson, A. S. Stochastic theory of early viral infection: Continuous versus burst production of virions. *PLoS Comput Biol* **7**(2), e1001058 (2011).

[3] Antia, R., Regoes, R. R., Koella, J. C., & Bergstrom, C. T. The role of evolution in the emergence of infectious diseases. *Nature* **426**(6967), 658–661, December (2003).

[4] Lloyd-Smith, J. O., Schreiber, S. J., Kopp, P. E., & Getz, W. M. Superspreading and the effect of individual variation on disease emergence. *Nature* **438**(7066), 355–359 (2005).

[5] Weinberger, L. S., Burnett, J. C., Toettcher, J. E., Arkin, A. P., & Schaffer, D. V. Stochastic gene expression in a lentiviral positive-feedback loop: HIV-1 tat fluctuations drive phenotypic diversity. *Cell* **122**(2), 169–182, July (2005).

[6] Eriksson, S., *et al.* Comparative analysis of measures of viral reservoirs in HIV-1 eradication studies. *PLoS Pathog* **9**(2), e1003174 (2013).

[7] Karlin, S. & Taylor, H. E. *A First Course in Stochastic Processes*. Academic Press, San Diego, (1975).

[8] Abate, J., Choudhury, G. L., & Whitt, W. An introduction to numerical transform inversion and its application to probability models. In Computational Probability, Grassmann, W. K., editor, number 24 in International Series in Operations Research & Management Science, 257–323. Springer US (2000).

[9] Conway, J. M. & Coombs, D. A stochastic model of latently infected cell reactivation and viral blip generation in treated HIV patients. *PLoS Comput Biol* **7**(4), e1002033 (2011).

[10] Siliciano, J. D., *et al.* Long-term follow-up studies confirm the stability of the latent reservoir for HIV-1 in resting CD4+ T cells. *Nat. Med.* **9**(6), 727–728 (2003).

[11] Archin, N. M., *et al.* Measuring HIV latency over time: Reservoir stability and assessing interventions. In *21st Conference on Retroviruses and Opportunistic Infections*, 406 (CROI, Boston, MA, 2014).

[12] Luo, R., Piovoso, M. J., Martinez-Picado, J., & Zurakowski, R. HIV model parameter estimates from interruption trial data including drug efficacy and reservoir dynamics. *PLoS ONE* **7**(7), e40198 (2012).

[13] Ruiz, L., *et al.* Structured treatment interruption in chronically HIV-1 infected patients after long-term viral suppression. *AIDS* **14**(4), 397 (2000).

[14] Davey, Jr., R. T., *et al.* HIV-1 and T cell dynamics after interruption of highly active antiretroviral therapy (HAART) in patients with a history of sustained viral suppression. *Proc. Natl. Acad. Sci. USA* **96**(26), 15109–15114 (1999).

[15] Markowitz, M., *et al.* A novel antiviral intervention results in more accurate assessment of human immunodeficiency virus type 1 replication dynamics and T-cell decay in vivo. *J. Virol.* **77**(8), 5037–5038 (2003).

[16] Ribeiro, R. M., *et al.* Estimation of the initial viral growth rate and basic reproductive number during acute HIV-1 infection. *Journal of Virology* **84**(12), 6096 –6102 (2010).

[17] Rosenbloom, D. I. S., Hill, A. L., Rabi, S. A., Siliciano, R. F., & Nowak, M. A. Antiretroviral dynamics determines HIV evolution and predicts therapy outcome. *Nat. Med.* **18**(9), 1378–1385 (2012).

[18] Ruiz, L., *et al.* HIV dynamics and t-cell immunity after three structured treatment interruptions in chronic HIV-1 infection. *AIDS* **15**(9), F19F27 (2001).

[19] Hofacre, A., Wodarz, D., Komarova, N. L., & Fan, H. Early infection and spread of a conditionally replicating adenovirus under conditions of plaque formation. *Virology* **423**(1), 89–96 (2012). PMID: 22192628.

[20] Sigal, A., *et al.* Cell-to-cell spread of HIV permits ongoing replication despite antiretroviral therapy. *Nature* **477**(7362), 95–98 (2011).

[21] Laird, G. M., *et al.* Rapid quantification of the latent reservoir for HIV-1 using a viral outgrowth assay. *PLoS Pathog* **9**(5), e1003398 (2013). PMID: 23737751 PMCID: PMC3667757.

[22] Pennings, P. S. Standing genetic variation and the evolution of drug resistance in HIV. *PLoS Comput Biol* **8**(6), e1002527 (2012).

[23] Kouyos, R. D., Althaus, C. L., & Bonhoeffer, S. Stochastic or deterministic: what is the effective population size of HIV-1? *Trends Microbiol* **14**(12), 507–511 (2006).

[24] Pennings, P. S., Kryazhimskiy, S., & Wakeley, J. Loss and recovery of genetic diversity in adapting populations of HIV. *PLoS Genetics* **10**(1), e1004000 (2014).

[25] Rouzine, I. M. & Coffin, J. M. Linkage disequilibrium test implies a large effective population number for HIV in vivo. *Proc. Natl. Acad. Sci. USA* **96**(19), 10758–10763 (1999).

[26] Rouzine, I. M., Coffin, J. M., & Weinberger, L. S. Fifteen years later: hard and soft selection sweeps confirm a large population number for HIV in vivo. *PLoS Genetics* **10**(2), e1004179 (2014).

[27] Singh, A., Razooky, B., Cox, C. D., Simpson, M. L., & Weinberger, L. S. Transcriptional bursting from the HIV-1 promoter is a significant source of stochastic noise in HIV-1 gene expression. *Biophysical journal* **98**(8), L32–34, April (2010).

[28] De Boer, R. J., Ribeiro, R. M., & Perelson, A. S. Current estimates for HIV-1 production imply rapid viral

clearance in lymphoid tissues. *PLoS Comput Biol* **6**(9), e1000906 (2010).

[29] Di Mascio, M., *et al.* Noninvasive in vivo imaging of CD4 cells in simian-human immunodeficiency virus (SHIV)-infected nonhuman primates. *Blood* **114**(2), 328–337 (2009).

[30] Ganusov, V. V. & De Boer, R. J. Do most lymphocytes in humans really reside in the gut? *Trends Immunol* **28**(12), 514–518 (2007).

[31] Chen, H. Y., Di Mascio, M., Perelson, A. S., Ho, D. D., & Zhang, L. Determination of virus burst size in vivo using a single-cycle SIV in rhesus macaques. *Proc. Natl. Acad. Sci. USA* **104**(48), 19079–19084 (2007).

[32] Reilly, C., Wietgrefe, S., Sedgewick, G., & Haase, A. Determination of simian immunodeficiency virus production by infected activated and resting cells. *AIDS* **21**(2), 163–168 (2007).

# Supplementary Figures

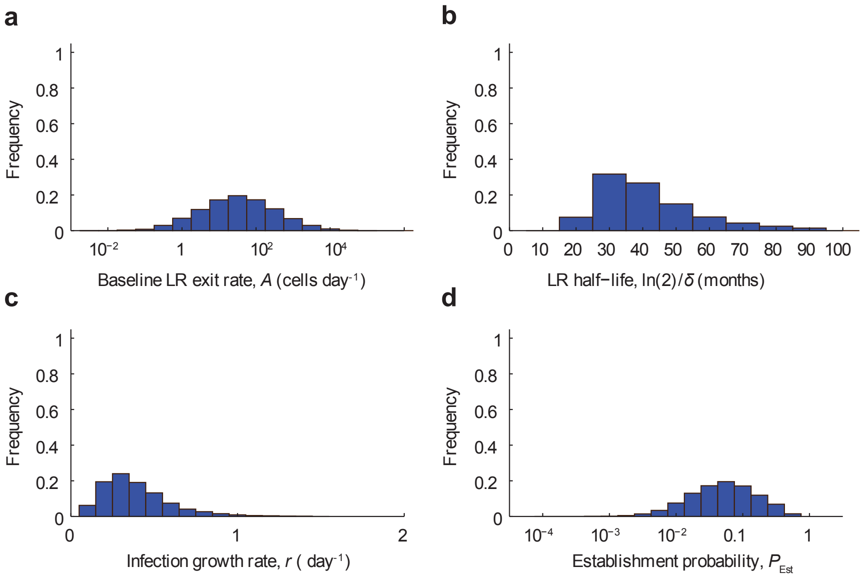


**Figure S1:** Parameter distributions described in Table 1 and used for results in Figs. 3a (uncertainty analysis) and 4 (target LRA efficacy). (A) LR exit rate prior to LRA therapy, (B) LR half-life, (C) infection growth rate, (D) establishment probability.

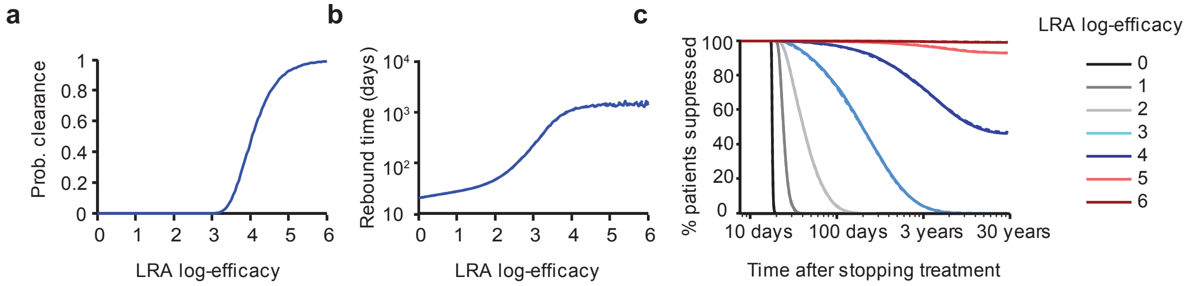


**Figure S2:** Comparing model predictions from the constant burst model (solid lines) with the basic (Poisson burst) model (dotted lines). For both models $r = 0.4$ d$^{-1}$, $A = 57$ cells d$^{-1}$, $\delta = 5.23 \times 10^{-4}$ d$^{-1}$, $P_{Est} = 0.07$. For each model all patients have the same underlying viral dynamic parameters: constant burst $b = 0.1273$ d$^{-1}$, $d = 0.8727$ d$^{-1}$, $\lambda = 11$; Poisson burst $b = 0.137$ d$^{-1}$, $d = 0.863$ d$^{-1}$, $\lambda = 10.22$; both $a = 5.7 \times 10^{-5}$ d$^{-1}$, $d_z = 4.66 \times 10^{-4}$ d$^{-1}$. a) Probability that the LR is cleared by LRA. Clearance occurs if all cells in the LR die before a reactivating lineage leads to viral rebound. b) Median viral rebound times (logarithmic scale), among patients who do not clear the infection. c) Survival curves (Kaplan-Meier plots) show the percentage of patients who have not yet experienced viral rebound, plotted as a function of the time (logarithmic scale) after treatment interruption. All simulations included $10^4$ to $10^5$ patients. Lack of visible dashed lines indicates both models give indistinguishable results.

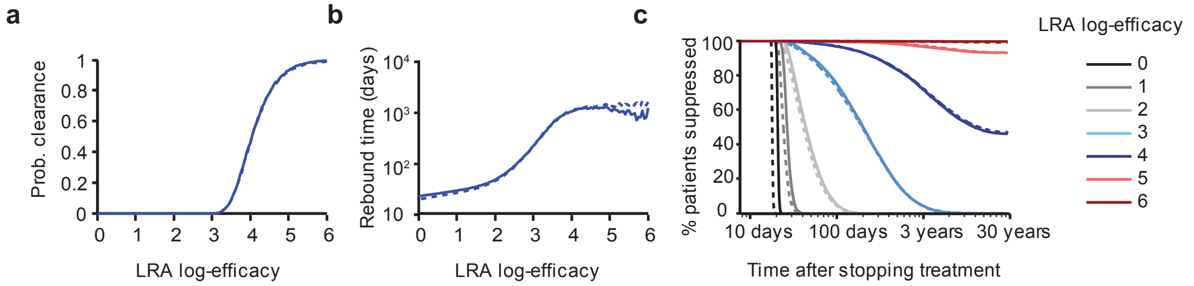


**Figure S3:** Comparing model predictions from the eclipse phase model (solid lines) with the basic (Poisson burst) model (dotted lines). For both models $r = 0.4$ d$^{-1}$, $A = 57$ cells d$^{-1}$, $\delta = 5.23 \times 10^{-4}$ d$^{-1}$, $P_{Est} = 0.07$. For each model all patients have the same underlying viral dynamic parameters: eclipse phase $b = 0.0952$ , $d = 0.9048$ , $\lambda = 29$, $e = 0.5$ d$^{-1}$, $f = 0.1$ d$^{-1}$; Poisson burst $b = 0.137$ d$^{-1}$, $d = 0.863$ d$^{-1}$, $\lambda = 10.22$; both $a = 5.7 \times 10^{-5}$ d$^{-1}$, $d_z = 4.66 \times 10^{-4}$ d$^{-1}$. a) Probability that the LR is cleared by LRA. Clearance occurs if all cells in the LR die before a reactivating lineage leads to viral rebound. b) Median viral rebound times (logarithmic scale), among patients who do not clear the infection. c) Survival curves (Kaplan-Meier plots) show the percentage of patients who have not yet experienced viral rebound, plotted as a function of the time (logarithmic scale) after treatment interruption. All simulations included $10^4$ to $10^5$ patients. Lack of visible dashed lines indicates both models give indistinguishable results.

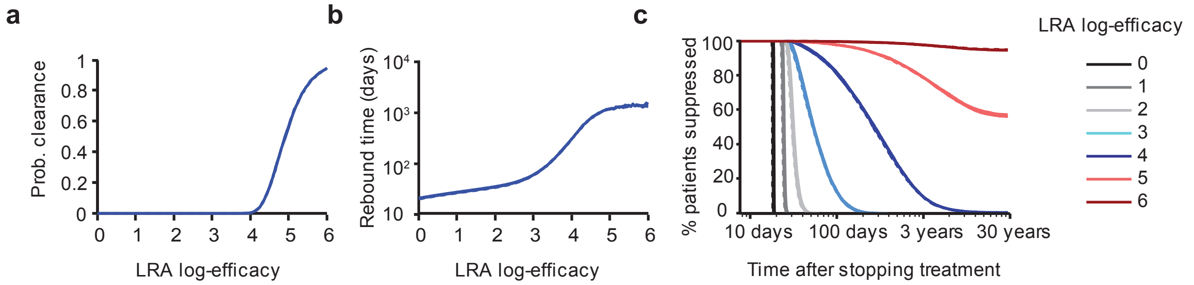


**Figure S4:** Comparing model predictions from two variations of the free virus model (solid lines) with the basic (Poisson burst) model (dotted lines). For both models $r = 0.4$ d$^{-1}$, $A = 57$ cells d$^{-1}$, $\delta = 5.23 \times 10^{-4}$ d$^{-1}$, $P_{Est} = 0.51$. For each model all patients have the same underlying viral dynamic parameters: free virus 1) $N = 10$, $k = 0.92$ d$^{-1}$, $d = 0.08$ d$^{-1}$, $b = 3.6$ d$^{-1}$, $c = 20$ d$^{-1}$; 2) $N = 1000$, $k = 0.997$ d$^{-1}$, $d = 0.0028$ d$^{-1}$, $b = 0.028$ d$^{-1}$, $c = 20$; Poisson burst $b = 1$, $d = 0$, $\lambda = 1.4$; both $a = 5.7 \times 10^{-5}$ d$^{-1}$, $d_z = 4.66 \times 10^{-4}$ d$^{-1}$. a) Probability that the LR is cleared by LRA. Clearance occurs if all cells in the LR die before a reactivating lineage leads to viral rebound. b) Median viral rebound times (logarithmic scale), among patients who do not clear the infection. c) Survival curves (Kaplan-Meier plots) show the percentage of patients who have not yet experienced viral rebound, plotted as a function of the time (logarithmic scale) after treatment interruption. All simulations included $10^4$ to $10^5$ patients. Lack of visible dashed lines and distinguishable solid lines indicates that the three models give indistinguishable results.

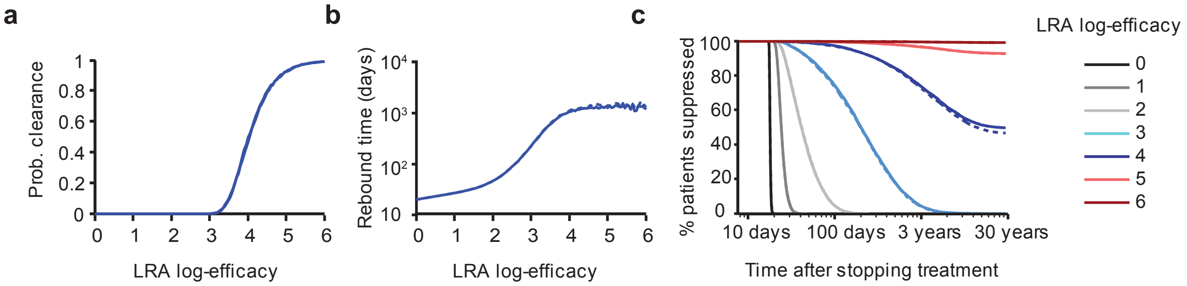


**Figure S5:** Comparing model predictions from the homeostatic proliferation model (solid lines) with the basic (Poisson burst) model (dotted lines). For both models $r = 0.4$ d$^{-1}$, $A = 57$ cells d$^{-1}$, $\delta = 5.23 \times 10^{-4}$ d$^{-1}$, $P_{Est} = 0.069$. For each model all patients have the same underlying viral dynamic parameters: homeostatic proliferation model $p = 3.3 \times 10^{-3}$ d$^{-1}$, $d_z = 3.8 \times 10^{-3}$ d$^{-1}$; Poisson burst $d_z = 4.66 \times 10^{-4}$ d$^{-1}$; both $b = 0.1346$ d$^{-1}$, $d = 0.8654$ d$^{-1}$, $\lambda = 10.4$, $a = 5.7 \times 10^{-5}$ d$^{-1}$. a) Probability that the LR is cleared by LRA. Clearance occurs if all cells in the LR die before a reactivating lineage leads to viral rebound. b) Median viral rebound times (logarithmic scale), among patients who do not clear the infection. c) Survival curves (Kaplan-Meier plots) show the percentage of patients who have not yet experienced viral rebound, plotted as a function of the time (logarithmic scale) after treatment interruption. All simulations included $10^4$ to $10^5$ patients. Lack of visible dashed lines indicates both models give indistinguishable results.

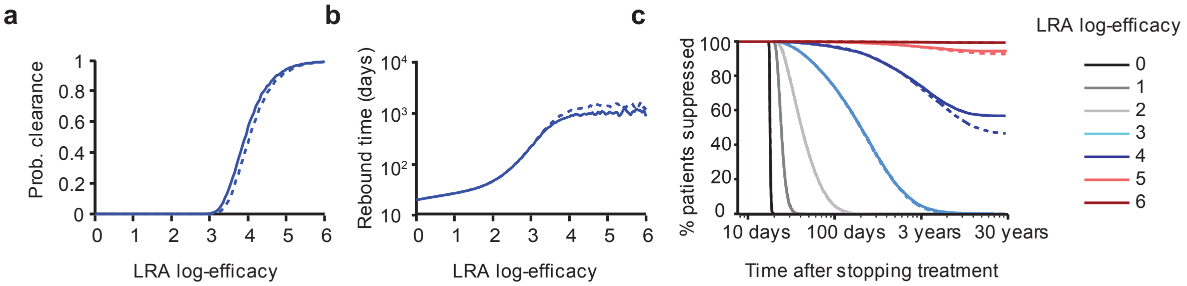


**Figure S6:** Comparing model predictions from the bursting homeostatic proliferation model (solid lines) with the basic (Poisson burst) model (dotted lines). For both models $r = 0.4$ d$^{-1}$, $A = 57$ cells d$^{-1}$, $\delta = 5.23 \times 10^{-4}$ d$^{-1}$, $P_{Est} = 0.069$. For each model all patients have the same underlying viral dynamic parameters: bursting homeostatic proliferation model $p = 2.2 \times 10^{-4}$ d$^{-1}$, $h = 4$, $d_z = 3.8 \times 10^{-3}$ d$^{-1}$; Poisson burst $d_z = 4.66 \times 10^{-4}$ d$^{-1}$; both $b = 0.1346$ d$^{-1}$, $d = 0.8654$ d$^{-1}$, $\lambda = 10.4$, $a = 5.7 \times 10^{-5}$ d$^{-1}$. a) Probability that the LR is cleared by LRA. Clearance occurs if all cells in the LR die before a reactivating lineage leads to viral rebound. b) Median viral rebound times (logarithmic scale), among patients who do not clear the infection. c) Survival curves (Kaplan-Meier plots) show the percentage of patients who have not yet experienced viral rebound, plotted as a function of the time (logarithmic scale) after treatment interruption. All simulations included $10^4$ to $10^5$ patients. Lack of visible dashed lines indicates both models give indistinguishable results.

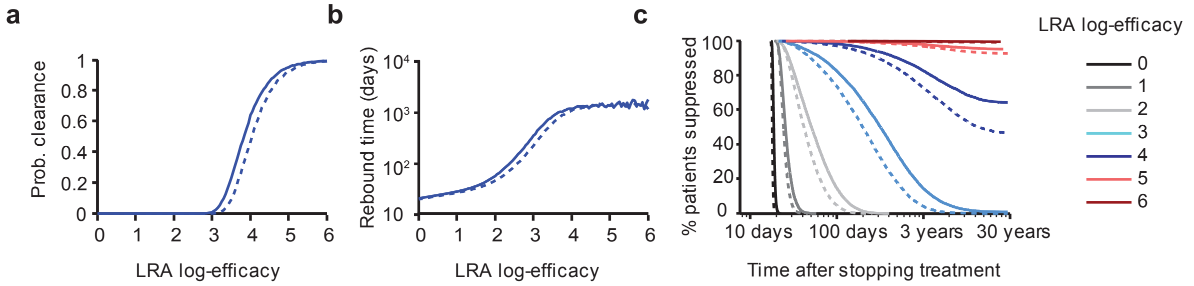


**Figure S7:** Comparing model predictions from the expansion upon reactivation model (solid lines) with the basic (Poisson burst) model (dotted lines). For both models $r = 0.4$ d$^{-1}$, $A = 57$ cells d$^{-1}$, $\delta = 5.23 \times 10^{-4}$ d$^{-1}$, $P_{Est} = 0.069$. For each model all patients have the same underlying viral dynamic parameters: expansion upon reactivation model $m = 4$, $a = 3.56 \times 10^{-6}$ d$^{-1}$; Poisson burst $a = 5.7 \times 10^{-5}$ d$^{-1}$; both $b = 0.1346$ d$^{-1}$, $d = 0.8654$ d$^{-1}$, $\lambda = 10.4$, $d_z = 4.66 \times 10^{-4}$ d$^{-1}$. a) Probability that the LR is cleared by LRA. Clearance occurs if all cells in the LR die before a reactivating lineage leads to viral rebound. b) Median viral rebound times (logarithmic scale), among patients who do not clear the infection. c) Survival curves (Kaplan-Meier plots) show the percentage of patients who have not yet experienced viral rebound, plotted as a function of the time (logarithmic scale) after treatment interruption. All simulations included $10^4$ to $10^5$ patients.
